# Supplementary material for: Learning What to Forget: Improving LLM Unlearning via Learned Token-Level Importance
Source: arXiv:2606.06320 source file (2026-06-04)
Supplement: Supplementary file 1 [file D-additional-experiments-bk.tex]

\section{Additional Experiments}\label{app:sec:additional-experiments}

This appendix collects experiments that support, but did not fit into,
the main paper. \Cref{app:subsec:additional:ablations} ablates the
design choices that compose \method{ATWU}---which parts of the
training paradigm, of the regulariser set, and of the
update schedule are actually necessary---using
\dataset{TOFU} \texttt{forget10} on \model{Llama-3.2-1B-Instruct} as
the test bed. \Cref{app:subsec:additional:augment} then takes the
opposite direction: rather than ablating \method{ATWU}, we plug the
\emph{learned scorer} into five existing forget objectives
(\method{SatImp}, \method{DPO}, \method{NPO}, \method{SimNPO},
\method{WGA}) and check whether the per-token weighting it provides
improves them.

% =====================================================================
\subsection{Scorer Ablations}\label{app:subsec:additional:ablations}

\paragraph{Setup.} All ablations in this subsection share the same
backbone, dataset, and trainer. We use \model{Llama-3.2-1B-Instruct}
on \dataset{TOFU} \texttt{forget10}, the largest forget split, and
\method{ATWU}'s alternating-update trainer with the
Bayesian-tuned hyperparameters of \cref{tab:hp-tofu-selected}.
The \emph{baseline} of every comparison is therefore the same
\method{ATWU} run that ships in our headline tables, i.e.\ jointly
training the scorer and the model with the regulariser set
$(\lambda_H, \lambda_\rho, \lambda_{\ell_2}) = (1, 10, 1)$ and updating the
scorer every model step.
Ablations are organised in three groups: \emph{scorer-state}
ablations (\cref{app:subsec:additional:ablations:state}) probe what
the trained scorer represents and how it interacts with the model;
\emph{architectural} ablations
(\cref{app:subsec:additional:ablations:arch}) test whether the
overall training paradigm---the bilevel formulation and the explicit
retain term---is necessary; and \emph{sweeps}
(\cref{app:subsec:additional:ablations:sweeps}) vary one
hyperparameter at a time over a small grid.

\subsubsection{Scorer-state ablations}\label{app:subsec:additional:ablations:state}

These four ablations leave the trainer untouched and only change
\emph{which scorer} the language model sees during unlearning. They
isolate the effect of the scorer-trajectory itself from the
optimisation procedure that produced it.

\paragraph{Trace.}
We checkpoint the scorer at initialisation (step $0$),
every $10$ model steps, and at the end of training, and rerun
evaluation against each snapshot. \emph{Why ablate.} The baseline
hides the temporal evolution of the scorer behind a single final
checkpoint; the trace lets us inspect whether the early-training
weights are already useful and whether the score distribution
stabilises before the final epoch. \emph{Design choice supported.} The
trace shows that the scorer's classification of forget-relevant
tokens is recognisable well before training ends and only sharpens
afterwards, which justifies the warm-start and frozen variants below.

\paragraph{Frozen-trained.}
We load the final scorer weights from the baseline run, freeze them,
and retrain the language model from scratch under that fixed
weighting. \emph{Why ablate.} If the converged scorer is already a
good standalone token classifier, retraining the model under it
should match the baseline; if the joint dynamics are essential, we
should observe a measurable gap. \emph{Design choice supported.} A
near-baseline result certifies that the converged scorer captures the
target token-relevance signal and is not merely a projection of the
specific model trajectory it co-trained with, justifying its use as
an interpretable readout of token importance.

\paragraph{Pretrain-frozen.}
We pretrain a fresh scorer for one epoch on the
\emph{original} (un-unlearned) model, then freeze it and run
unlearning. \emph{Why ablate.} This isolates the contribution of the
``clean'' importance signal---the one available before the model
starts moving away from $\thpre$---from the contribution of online
co-adaptation during unlearning. \emph{Design choice supported.}
A drop relative to the baseline shows that the scorer must keep
tracking the model as it changes, motivating the alternating
formulation rather than a one-shot offline label.

\paragraph{Pretrain-unfrozen.}
Identical pretraining, but the scorer is then fine-tuned online
during unlearning, i.e.\ a warm-started version of the baseline.
\emph{Why ablate.} It separates the cost of cold-starting the scorer
from the value of co-adaptation. \emph{Design choice supported.}
If pretrain-unfrozen matches or slightly exceeds the baseline at the
same compute budget, the cold start is not a bottleneck; if it
overshoots and then degrades, the cold-start regularises the scorer
toward a useful fixed point and pretraining is unnecessary.

\subsubsection{Architectural ablations}\label{app:subsec:additional:ablations:arch}

\paragraph{No retain ($\alpha = 0$).}
We drop the retain term $\alpha\,\mathcal{L}_{\mathrm{R}}$ from the
main objective entirely and rerun a fresh hyperparameter search,
since removing $\alpha$ shifts the optimum of the remaining
parameters. \emph{Why ablate.} The scorer's gating already protects
retain knowledge by zeroing out structural tokens; the retain term is
a redundant safety net only if that gating is reliable. \emph{Design
choice supported.} The no-retain run lets us decide whether the
explicit retain regulariser earns its place in
\eqref{eq:atwu} or whether the scorer subsumes it.

\paragraph{Joint training.}
Instead of the alternating formulation of
\cref{alg:atwu}, we collapse the two updates into a single
backward pass: the scorer parameters live in the main optimiser, the
regularisers fold into the main loss, and there is no separate scorer
trainer. \emph{Why ablate.} Bilevel training is the more invasive
choice; if a flat joint formulation matches it, the separation is
unnecessary engineering. \emph{Design choice supported.} A gap to the
baseline justifies the alternating procedure introduced in
\cref{sec:setting} and \cref{alg:atwu}, and pinpoints which loss
component (the scorer regularisers vs.\ the model objective) needs
its own optimiser to behave well.

\subsubsection{Sweeps}\label{app:subsec:additional:ablations:sweeps}

\paragraph{Regulariser combinations.}
We toggle each of the three scorer regularisers
$(\lambda_H, \lambda_\rho, \lambda_{\ell_2})$ between
``off'' ($0$) and ``on'' (its baseline value
$1, 10, 1$ respectively), giving a $2^3 = 8$-cell grid.
\emph{Why ablate.} Every regulariser carries a cost, both in
hyperparameters and in conceptual machinery, and we want to credit
only those that move the metrics. \emph{Design choice supported.}
The sweep narrows the regulariser set down to those that
\emph{individually} contribute to the final FQ/RD/UQ gap, which we
then keep in the main objective. The remainder are reported here for
transparency but excluded from the headline configuration.

\paragraph{Update frequency.}
We vary how often the scorer is updated relative to the model,
$n \in \{1, 5, 10\}$ where $n = 1$ updates the scorer at every model
step and $n = 10$ updates it once per ten model steps.
\emph{Why ablate.} Updating the scorer more often is cheap on a
single linear layer but can amplify noise in early-training
gradients; updating less often is closer to a frozen-scorer
schedule. \emph{Design choice supported.} The sweep shows how stale
the scorer can be before the alternating formulation degenerates,
and locates a plateau that motivates the value used in the headline
configuration.

\paragraph{Consolidated table.} The full panel of results for every
ablation in this subsection is reported in
\cref{tab:ablation-tofu-1b-f10}, where rows are grouped by the
ablation family. Throughout the table we use the same column layout
and best/second-best emphasis as the headline tables of
\cref{app:subsec:exp:unlearning}, with the unmodified
\method{ATWU} baseline included at the top of each block for
reference.

\begin{center}\itshape\small
{[\textbf{TODO}: insert \texttt{tab:ablation-tofu-1b-f10} here. The
36 rows live in the ablation-results json (1B, forget10);
FQ/RD/UQ are derived from per-row $\mathcal{J}_\mathrm{W}$ and
$\mathcal{J}_\mathrm{AVG}$ against the original-model baselines
$\mathcal{J}_\mathrm{W}^\mathrm{orig}=0.9314$,
$\mathcal{J}_\mathrm{AVG}^\mathrm{orig}=0.4298$.]}
\end{center}

% =====================================================================
\subsection{Augmenting Existing Unlearning Methods}\label{app:subsec:additional:augment}

The scorer learned by \method{ATWU} is, at heart, a per-token weight
in $(0, 1)$. Nothing about the way we train it ties it specifically
to the gradient-difference forget objective: any forget loss that
already operates token-wise can, in principle, multiply or modulate
its summands by the scorer. In this subsection we test that claim by
plugging the scorer into five widely-used forget objectives and
re-running the full \dataset{TOFU} pipeline. We obtain the augmented
methods with no architectural changes; only the forget term changes.
\todo{cross-ref the methodology section once it is finalised.}

\paragraph{Notation.}
For a forget input $x \in \DF$ with target tokens of length $T$ and
a current model $\tth$ with frozen reference $\thpre$, write
\begin{align*}
    \ell_t &\;\defeq\; \lR(\tth,\prefix{x}{t})
        = -\log p_{\tth}(x_t \mid \prefix{x}{t-1}), \\
    g_t   &\;\defeq\; \zhjx \quad\text{at position } t \in [T],
\end{align*}
and let $M_t \in \{0,1\}$ be the standard valid-target mask
(zero on prompt and padding tokens). We use the saturation
shorthand $\mathrm{sat}(u) = e^{-u}$ and define $|M| = \sum_t M_t$.
Each method's full objective has the form
$\mathcal{L} = \alpha\,\mathcal{L}_{\mathrm{retain}} +
\gamma\,\mathcal{L}_{\mathrm{forget}}$; only
$\mathcal{L}_{\mathrm{forget}}$ changes under augmentation, so we
display only that term and write $\mathcal{L}_{\mathrm{forget}}^m$
for method $m$ in its original form and
$\widetilde{\mathcal{L}}_{\mathrm{forget}}^m$ for the augmented
version. All other components, including the retain loss
$\mathcal{L}_{\mathrm{retain}}$ and the per-method
hyperparameters, are kept identical to those reported in
\cref{tab:hp-tofu-selected}.

\subsubsection{SatImp / GradDiff Family}

\citet{yang2025exploring} introduce \method{SatImp} as a
saturated, importance-weighted variant of gradient difference.
With a generic per-token importance heuristic
$w_t \in [0, 1]$ (typically derived from token probability or loss),
the original forget loss reads
\begin{equation}
    \mathcal{L}_{\mathrm{forget}}^{\method{SatImp}}
    \;=\; -\frac{1}{|M|}\sum_t M_t\, w_t\,
        \bigl(\mathrm{sat}(w_t \, \ell_t)\bigr)^{\beta}\, \ell_t
    \;=\; -\frac{1}{|M|}\sum_t M_t\, w_t\,
        e^{-\beta w_t \ell_t}\, \ell_t.
\end{equation}
The score $w_t$ acts \emph{both} multiplicatively, gating the
contribution of each token, \emph{and} inside the saturation argument,
making the down-weighting bite earlier on highly-scored tokens. The
\method{ATWU} augmentation simply replaces the heuristic $w_t$ with
the learned $g_t$:
\begin{equation}
    \widetilde{\mathcal{L}}_{\mathrm{forget}}^{\method{SatImp}}
    \;=\; -\frac{1}{|M|}\sum_t M_t\, g_t\,
        e^{-\beta g_t \ell_t}\, \ell_t.
\end{equation}
The structural role of the weight is unchanged; only its source---a
fixed proxy vs.\ a learned linear scorer over hidden states---differs.

\subsubsection{DPO and NPO}

The \method{DPO} forget objective of \citet{rafailov2023direct}, as
adapted for unlearning by \citet{maini2024tofu}, contrasts the
sequence-level NLL of the original target $y^-$ (\emph{lose}) and an
alternate target $y^+$ (\emph{win}) under the current model and a
frozen reference. Writing
$\mathrm{NLL}_\theta(x, y) = \sum_t M_t\, \ell_t(y)$ and
$r_\bullet = -\bigl(\mathrm{NLL}_\theta(x, y^\bullet) -
\mathrm{NLL}_{\mathrm{ref}}(x, y^\bullet)\bigr)$,
\begin{equation}
    \mathcal{L}_{\mathrm{forget}}^{\method{DPO}}
    \;=\; -\frac{2}{\beta}\,\mathbb{E}\!\left[
        \log \sigma\bigl(\beta\,(r_{\mathrm{win}} - r_{\mathrm{lose}})\bigr)
    \right].
\end{equation}
\method{NPO}~\citep{zhang2024negative} is the special case
$r_{\mathrm{win}} \equiv 0$, i.e.\ it discards the alternate target
and leans entirely on the lose-side log-ratio.

We augment both objectives in the same way: replace the lose-side
NLL with a \emph{scored} NLL that re-weights its summands by $g_t$,
while leaving the win side and the reference NLL untouched. To
preserve the magnitude of the resulting log-ratio, we rescale the
weights so that $\sum_t w_t M_t = T$, giving
\begin{equation}
    w_t \;=\; \frac{2 g_t \cdot T}{\sum_s 2 g_s\, M_s},
    \qquad
    \mathrm{NLL}^{\mathrm{scored}}_\theta(x, y)
    \;=\; \sum_t M_t\, w_t\, \ell_t(y),
\end{equation}
and use $\widetilde{r}_{\mathrm{lose}}
= -(\mathrm{NLL}^{\mathrm{scored}}_\theta(x, y^-) -
\mathrm{NLL}_{\mathrm{ref}}(x, y^-))$ in place of $r_{\mathrm{lose}}$.
The win-side reward and the reference NLL are held fixed, so the
augmentation only shifts \emph{where} the lose-side mass is
concentrated across tokens; the overall scale is preserved.

\subsubsection{SimNPO}

\method{SimNPO}~\citep{fan2024simplicity} drops the reference model
and length-normalises the lose-side NLL directly, replacing the
log-ratio of \method{NPO} with a margin-shifted score
\begin{equation}
    s(x, y)
    \;=\; \frac{1}{|M|}\sum_t M_t\, \ell_t \;-\; \delta,
    \qquad
    \mathcal{L}_{\mathrm{forget}}^{\method{SimNPO}}
    \;=\; -\frac{2}{\beta}\,\mathbb{E}\!\left[
        \log \sigma(\beta\,s)
    \right].
\end{equation}
Because the score is already length-normalised, no extra rescaling is
required: we simply re-weight the summands by $2 g_t$,
\begin{equation}
    \widetilde{s}(x, y)
    \;=\; \frac{1}{|M|}\sum_t M_t\,(2 g_t)\,\ell_t \;-\; \delta,
    \qquad
    \widetilde{\mathcal{L}}_{\mathrm{forget}}^{\method{SimNPO}}
    \;=\; -\frac{2}{\beta}\,\mathbb{E}\!\left[
        \log \sigma(\beta\,\widetilde{s})
    \right].
\end{equation}
The factor $2$ keeps the per-token weight at the un-augmented value
when $g_t = \tfrac{1}{2}$, the scorer's initialisation
(\cref{prop:init}), so the augmented objective coincides with the
original at the start of training.

\subsubsection{WGA}

\method{WGA}~\citep{wang2025rethinking} uses a saturation-only forget
loss with no explicit importance weight,
\begin{equation}
    \mathcal{L}_{\mathrm{forget}}^{\method{WGA}}
    \;=\; -\frac{1}{|M|}\sum_t M_t\,
        \bigl(\mathrm{sat}(\ell_t)\bigr)^{\beta}\, \ell_t
    \;=\; -\frac{1}{|M|}\sum_t M_t\,
        e^{-\beta \ell_t}\, \ell_t.
\end{equation}
We augment \method{WGA} by injecting $g_t$ \emph{exclusively} into the
saturation exponent: we replace $\beta$ with $\beta \cdot 2 g_t$,
\begin{equation}
    \widetilde{\mathcal{L}}_{\mathrm{forget}}^{\method{WGA}}
    \;=\; -\frac{1}{|M|}\sum_t M_t\,
        \bigl(\mathrm{sat}(\ell_t)\bigr)^{\beta \cdot 2 g_t}\, \ell_t
    \;=\; -\frac{1}{|M|}\sum_t M_t\,
        e^{-2 \beta g_t \ell_t}\, \ell_t.
\end{equation}
Tokens flagged as forget-relevant ($g_t \to 1$) experience a sharper
saturation gate and are therefore down-weighted aggressively once
they become confident, while structural tokens
($g_t \to 0$) revert to a near-uniform cross-entropy ascent. The
scaling by $2$ again pins the augmentation to the original objective
at scorer initialisation.

\paragraph{Where $g_t$ enters, at a glance.}
\Cref{tab:augment-glance} summarises, for each method, the
structural role $g_t$ plays in the forget loss. \method{SatImp}
remains the only method in which $g_t$ is used twice: as a gate and
inside the saturation. The DPO-family augmentations all use $g_t$ as
a linear per-token weight inside the log-ratio (or its
length-normalised cousin), and \method{WGA} is the only method for
which $g_t$ enters \emph{exclusively} through the saturation
exponent.

\begin{table}[t]
    \centering
    \small
    \captionsetup{justification=centering}
    
    \begin{tabular}{@{}l l@{}}
        \toprule
        \textbf{Method} & \textbf{Role of $g_t$ in $\mathcal{L}_{\mathrm{forget}}$} \\
        \midrule
        \method{SatImp} &
            multiplicative gate \emph{and} inside saturation:
            $g_t\, e^{-\beta g_t \ell_t}\, \ell_t$ \\
        \method{DPO}    &
            rescaled per-token weight $w_t \propto g_t$ on the
            \emph{lose} NLL inside the log-ratio \\
        \method{NPO}    &
            same as \method{DPO}, with $r_{\mathrm{win}} \equiv 0$ \\
        \method{SimNPO} &
            per-token weight $2 g_t$ on $\ell_t$ before length
            normalisation \\
        \method{WGA}    &
            modulates the saturation exponent only:
            $e^{-2 \beta g_t \ell_t}\, \ell_t$ \\
        \bottomrule
    \end{tabular}
    \vspace{0.5em}
    \caption{Where the learned scorer $g_t$ enters the forget loss in
    each augmented method.}
    \label{tab:augment-glance}
\end{table}

\paragraph{Results.}
\Cref{tab:augment-tofu-1b-f10} reports the full
\dataset{TOFU} \texttt{forget10} panel (\model{Llama-3.2-1B-Instruct})
for each baseline \emph{and} its scorer-augmented variant, using the
same metric layout as \cref{tab:tofu-full-1b-f10}.
\Cref{fig:augment-uplift-pp} visualises the percentage-point
movement of FQ, RD, and UQ when each baseline is replaced by its
augmented counterpart: positive bars on FQ/UQ and negative bars on
RD indicate that the scorer translates into actual gains on that axis
without retain-side cost.

\begin{center}\itshape\small
{[\textbf{TODO}: insert \texttt{tab:augment-tofu-1b-f10} here,
sourced from the final-runs json (forget10, 1B). Pair each
baseline (DPO, NPO, SimNPO, WGA, GradDiff/SatImp) with its
SB-counterpart and derive FQ/RD/UQ from $\mathcal{J}_\mathrm{W}$,
$\mathcal{J}_\mathrm{AVG}$ against
$\mathcal{J}_\mathrm{W}^\mathrm{orig}=0.9314$,
$\mathcal{J}_\mathrm{AVG}^\mathrm{orig}=0.4298$.]}
\end{center}

\begin{figure}[H]
    \centering
    \fbox{\parbox[c][0.22\linewidth][c]{0.85\linewidth}{\centering
        \emph{[figure placeholder: pp-uplift bar chart. Drop the
        asset at \texttt{content/figures/scorer\_uplift\_pp.pdf}
        and uncomment the \texttt{\textbackslash includegraphics}
        line above.]}
    }}
    \caption{Percentage-point change in FQ, RD, and UQ when each
    baseline forget objective is replaced by its scorer-augmented
    variant on \dataset{TOFU} \texttt{forget10}
    (\model{Llama-3.2-1B-Instruct}). Positive values on FQ/UQ and
    negative values on RD reflect a scorer-induced improvement.}
    \label{fig:augment-uplift-pp}
\end{figure}
