# Supplementary material for: Learning What to Forget: Improving LLM Unlearning via Learned Token-Level Importance
Source: arXiv:2606.06320 source file (2026-06-04)
Supplement: Supplementary file 2 [file A-notation.tex]

\section{Notation and Preliminaries}

we ref \autoref{sec:intro}.
