# Supplementary material for: Learning What to Forget: Improving LLM Unlearning via Learned Token-Level Importance
Source: arXiv:2606.06320 source file (2026-06-04)
Supplement: Supplementary file 4 [file F-prompts.tex]

\section{Prompts and Judge Rubrics}\label{app:sec:prompts}
