# Supplementary material for: Learning What to Forget: Improving LLM Unlearning via Learned Token-Level Importance
Source: arXiv:2606.06320 source file (2026-06-04)
Supplement: Supplementary file 5 [file Z-backup.tex]

% For things we want to keep just in case but don't want to cluter the other files


% Alternative layout: horizontal dataset labels on top (for comparison).
% \begin{table}[t]
%     \centering
%     \small
%     \renewcommand{\arraystretch}{1.2}
%     \setlength{\dashlinedash}{0.7pt}\setlength{\dashlinegap}{1.8pt}
%     \resizebox{\textwidth}{!}{%
%     \begin{tabular}{@{}c ccc ccc :ccc ccc@{}}
%         \toprule
%         \multirow{3}{*}[-1.1ex]{\textbf{Method}}
%           & \multicolumn{6}{c}{\textbf{TOFU}}
%           & \multicolumn{6}{c}{\textbf{RWKU}} \\
%         \cmidrule(lr){2-7} \cmidrule(lr){8-13}
%           & \multicolumn{3}{c}{\textbf{Unlearning}} & \multicolumn{3}{c}{\textbf{Utility}}
%           & \multicolumn{3}{c}{\textbf{Unlearning}} & \multicolumn{3}{c}{\textbf{Utility}} \\
%         \cmidrule(lr){2-4} \cmidrule(lr){5-7} \cmidrule(lr){8-10} \cmidrule(lr){11-13}
%           & $\FQ\,\uparrow$ & $\RD\,\downarrow$ & $\UQ\,\uparrow$ & MMLU\,$\uparrow$ & Rep.\,$\uparrow$ & \WR
%           & $\FQ\,\uparrow$ & $\RD\,\downarrow$ & $\UQ\,\uparrow$ & MMLU\,$\uparrow$ & Rep.\,$\uparrow$ & \WR \\
%         \midrule
%         \method{Original} &$0.0$              & $0.0$              & $0.0$              & $66.6$             & $546$             & ---
%                           & $0.0$              & $0.0$              & $0.0$              & $70.1$             & $529$             & ---                \\
%         \midrule
%         \method{GradDiff} &$39.7$             & $17.3$             & $22.4$             & $66.1$             & $545$             & $48.0$
%                           & $81.9$             & $36.7$             & $45.2$             & $69.2$             & $514$             & $43.0$             \\
%         \method{DPO} &$59.5$             & $15.0$             & $44.5$             & $64.3$             & $533$             & $38.5$
%                           & $12.3$             & $\mathbf{17.0}$    & $0.0$              & $69.7$             & $523$             & $43.0$             \\
%         \method{NPO} &$48.0$             & $5.0$              & $43.0$             & $\underline{66.2}$ & $\underline{551}$ & $48.5$
%                           & $47.6$             & $39.1$             & $8.5$              & $68.1$             & $\mathbf{543}$    & $33.5$             \\
%         \method{SimNPO} &$69.3$             & $6.5$              & $62.8$             & $65.8$             & $541$             & $50.5$
%                           & $51.8$             & $29.7$             & $22.1$             & $68.8$             & $\underline{529}$ & $45.5$             \\
%         \method{JensUn} &$\mathbf{98.0}$    & $9.6$              & $\underline{88.3}$ & $65.3$             & $236$             & $11.0$
%                           & $\mathbf{85.4}$    & $36.1$             & $49.3$             & $\underline{70.2}$ & $523$             & $\mathbf{46.5}$    \\
%         \method{WGA} &$66.8$             & $4.8$              & $62.1$             & $66.0$             & $550$             & $\mathbf{60.0}$
%                           & $78.0$             & $26.1$             & $\underline{51.9}$ & $69.4$             & $518$             & $41.0$             \\
%         \method{SatImp} &$78.6$             & $\underline{3.0}$  & $75.6$             & $65.9$             & $549$             & $53.5$
%                           & $77.3$             & $29.3$             & $48.0$             & $69.8$             & $518$             & $40.0$             \\
%         \midrule
%         \method{Ours} &$\underline{92.0}$ & $\mathbf{2.1}$     & $\mathbf{89.8}$    & $\mathbf{66.4}$    & $\mathbf{558}$    & $\underline{54.5}$
%                           & $\underline{80.8}$ & $\underline{23.1}$ & $\mathbf{57.8}$    & $\mathbf{70.4}$    & $522$             & $\underline{46.0}$ \\
%         \bottomrule
%     \end{tabular}%
%     }
%     \vspace{0.5em}
%     \caption{Same as \cref{tab:headline-results}, but with the dataset labels rendered as horizontal group headers on top instead of rotated labels between the method and result columns.}
%     \label{tab:headline-results-horizontal}
% \end{table}

% \begin{table}[t]
%     \centering
%     \small
%     \renewcommand{\arraystretch}{1.2}
%     \resizebox{\textwidth}{!}{%
%     \begin{tabular}{@{}c c ccc ccc c ccc ccc@{}}
%         \toprule
%         \multirow{2}{*}[-0.4ex]{\textbf{Method}}
%           & & \multicolumn{3}{c}{\textbf{Unlearning}}
%           & \multicolumn{3}{c}{\textbf{Utility}}
%           & & \multicolumn{3}{c}{\textbf{Unlearning}}
%           & \multicolumn{3}{c}{\textbf{Utility}} \\
%         \cmidrule(lr){3-5} \cmidrule(lr){6-8} \cmidrule(lr){10-12} \cmidrule(lr){13-15}
%           & & $\FQ\,\uparrow$ & $\RD\,\downarrow$ & $\UQ\,\uparrow$ & MMLU\,$\uparrow$ & Rep.\,$\uparrow$ & \WR
%           & & $\FQ\,\uparrow$ & $\RD\,\downarrow$ & $\UQ\,\uparrow$ & MMLU\,$\uparrow$ & Rep.\,$\uparrow$ & \WR \\
%         \midrule
%         \method{Original} &\multirow{9}{*}{\rotatebox[origin=c]{90}{\texttt{Llama-3.2-1B-Instruct}}}
%                  & $0.0$              & $0.0$              & $0.0$              & $45.1$           & $559$             & ---
%                  & \multirow{9}{*}{\rotatebox[origin=c]{90}{\texttt{Llama-3.1-8B-Instruct}}}
%                  & $0.0$              & $0.0$              & $0.0$              & $66.6$           & $546$             & ---                \\
%         \midrule
%         \method{GradDiff} && $37.8$             & $13.0$             & $24.8$             & $\mathbf{45.2}$  & $563$             & $55.5$
%                  & & $39.7$             & $17.3$             & $22.4$             & $66.1$           & $545$             & $48.0$             \\
%         \method{DPO} && $42.8$             & $11.2$             & $31.6$             & $44.9$           & $560$             & $\mathbf{59.0}$
%                  & & $59.5$             & $15.0$             & $44.5$             & $64.3$           & $533$             & $38.5$             \\
%         \method{NPO} && $56.0$             & $\mathbf{1.4}$     & $54.6$             & $44.9$           & $563$             & $55.0$
%                  & & $48.0$             & $5.0$              & $43.0$             & $\underline{66.2}$ & $\underline{551}$ & $48.5$           \\
%         \method{SimNPO} && $38.3$             & $4.4$              & $33.9$             & $\underline{45.1}$ & $566$           & $\underline{57.0}$
%                  & & $69.3$             & $6.5$              & $62.8$             & $65.8$           & $541$             & $50.5$             \\
%         \method{JensUn} && $\mathbf{98.0}$    & $15.3$             & $\mathbf{82.8}$    & $45.1$           & $343$             & $23.5$
%                  & & $\mathbf{98.0}$    & $9.6$              & $\underline{88.3}$ & $65.3$           & $236$             & $11.0$             \\
%         \method{WGA} && $50.0$             & $8.5$              & $41.5$             & $45.0$           & $568$             & $56.0$
%                  & & $66.8$             & $4.8$              & $62.1$             & $66.0$           & $550$             & $\mathbf{60.0}$    \\
%         \method{SatImp} && $71.2$             & $4.1$              & $67.1$             & $44.8$           & $\underline{570}$ & $55.0$
%                  & & $78.6$             & $\underline{3.0}$  & $75.6$             & $65.9$           & $549$             & $53.5$             \\
%         \midrule
%         \method{Ours} && $\underline{77.2}$ & $\underline{3.5}$  & $\underline{73.7}$ & $44.9$           & $\mathbf{574}$    & $53.0$
%                  & & $\underline{92.0}$ & $\mathbf{2.1}$     & $\mathbf{89.8}$    & $\mathbf{66.4}$  & $\mathbf{558}$    & $\underline{54.5}$ \\
%         \bottomrule
%     \end{tabular}%
%     }
%     \vspace{0.5em}
%     \caption{Headline unlearning and utility results on \dataset{TOFU} \texttt{forget10} across the two base-model scales: \model{Llama-3.2-1B-Instruct} (left) and \model{Llama-3.1-8B-Instruct} (right). Conventions follow \cref{tab:headline-results}: all values are percentages except Rep., which is a count of repeated bi-/tri-grams; \FQ, \RD, \UQ are zero by definition for the Original row, whose \WR is undefined. In each performance column, excluding the Original row, the best score is in bold and the second best is underlined.}
%     \label{tab:headline-results-tofu-scales}
% \end{table}
